# Supplementary material for: Unextendible entanglement of quantum channels
Source: arXiv:2407.15944 ancillary file (2024-07-22)
Supplement: Supplementary file 1 [file Raw_data.pdf]

## Raw Data for the figures

In this file we present the raw data that was used to plot the figures in the main text. The code used to generate this raw data is also available with the arXiv posting.

### I. DATA FOR FIGURE 6

| Erasure probability (p) | q = 0.0 | q=0.1  | q = 0.2 | q=0.3  | q = 0.4 |
|-------------------------|---------|--------|---------|--------|---------|
| 0.0                     | 0.9999  | 0.9999 | 0.9998  | 0.9999 | 0.9999  |
| 0.0125                  | 0.9874  | 0.9658 | 0.9634  | 0.9624 | 0.9618  |
| 0.025                   | 0.9749  | 0.9364 | 0.9309  | 0.9279 | 0.9260  |
| 0.0375                  | 0.9624  | 0.9130 | 0.9004  | 0.8953 | 0.8919  |
| 0.05                    | 0.9499  | 0.8971 | 0.8710  | 0.8640 | 0.8590  |
| 0.0625                  | 0.9374  | 0.8839 | 0.8442  | 0.8336 | 0.8272  |
| 0.075                   | 0.9249  | 0.8707 | 0.8222  | 0.8040 | 0.7961  |
| 0.0875                  | 0.9124  | 0.8574 | 0.8039  | 0.7754 | 0.7656  |
| 0.1                     | 0.8999  | 0.8442 | 0.7887  | 0.7501 | 0.7357  |
| 0.1125                  | 0.8875  | 0.8311 | 0.7749  | 0.7280 | 0.7063  |
| 0.125                   | 0.8750  | 0.8178 | 0.7611  | 0.7084 | 0.6788  |
| 0.1375                  | 0.8625  | 0.8047 | 0.7472  | 0.6912 | 0.6540  |
| 0.15                    | 0.8500  | 0.7915 | 0.7334  | 0.6759 | 0.6315  |
| 0.1625                  | 0.8375  | 0.7783 | 0.7197  | 0.6616 | 0.6110  |
| 0.175                   | 0.8250  | 0.7651 | 0.7059  | 0.6473 | 0.5925  |
| 0.1875                  | 0.8125  | 0.7520 | 0.6921  | 0.6331 | 0.5756  |
| 0.2                     | 0.8000  | 0.7388 | 0.6784  | 0.6189 | 0.5603  |
| 0.2125                  | 0.7875  | 0.7256 | 0.6647  | 0.6048 | 0.5458  |
| 0.225                   | 0.7750  | 0.7124 | 0.6510  | 0.5906 | 0.5314  |
| 0.2375                  | 0.7625  | 0.6993 | 0.6373  | 0.5765 | 0.5170  |

## II. DATA FOR FIGURE 7

| Erasure prob. (p) | $\hat{E}_{\alpha(10)}^u(\mathcal{E}^P)$ (d = 2) | Analytical(d=2) | $\hat{E}_{\alpha(10)}^u(\mathcal{E}^P)$ (d = 3) | Analytical(d=3) |
|-------------------|-------------------------------------------------|-----------------|-------------------------------------------------|-----------------|
| 0.5000            | 0.0000                                          | 0.0000          | 0.0000                                          | 0.0000          |
| 0.4872            | 0.0010                                          | 0.0009          | 0.0009                                          | 0.0009          |
| 0.4744            | 0.0038                                          | 0.0038          | 0.0038                                          | 0.0038          |
| 0.4615            | 0.0086                                          | 0.0086          | 0.0086                                          | 0.0086          |
| 0.4487            | 0.0152                                          | 0.0152          | 0.0153                                          | 0.0152          |
| 0.4359            | 0.0239                                          | 0.0238          | 0.0239                                          | 0.0238          |
| 0.4231            | 0.0345                                          | 0.0344          | 0.0345                                          | 0.0344          |
| 0.4103            | 0.0470                                          | 0.0470          | 0.0470                                          | 0.0470          |
| 0.3974            | 0.0616                                          | 0.0616          | 0.0616                                          | 0.0616          |
| 0.3846            | 0.0783                                          | 0.0782          | 0.0783                                          | 0.0782          |
| 0.3718            | 0.0971                                          | 0.0970          | 0.0971                                          | 0.0970          |
| 0.3590            | 0.1181                                          | 0.1180          | 0.1181                                          | 0.1180          |
| 0.3462            | 0.1413                                          | 0.1412          | 0.1413                                          | 0.1412          |
| 0.3333            | 0.1668                                          | 0.1667          | 0.1668                                          | 0.1667          |
| 0.3205            | 0.1936                                          | 0.1935          | 0.1947                                          | 0.1946          |
| 0.3077            | 0.2207                                          | 0.2206          | 0.2252                                          | 0.2250          |
| 0.2949            | 0.2481                                          | 0.2480          | 0.2582                                          | 0.2580          |
| 0.2821            | 0.2758                                          | 0.2757          | 0.2940                                          | 0.2938          |
| 0.2692            | 0.3038                                          | 0.3037          | 0.3327                                          | 0.3324          |
| 0.2564            | 0.3321                                          | 0.3320          | 0.3745                                          | 0.3742          |
| 0.2436            | 0.3608                                          | 0.3607          | 0.4191                                          | 0.4188          |
| 0.2308            | 0.3898                                          | 0.3897          | 0.4650                                          | 0.4647          |
| 0.2179            | 0.4192                                          | 0.4191          | 0.5118                                          | 0.5115          |
| 0.2051            | 0.4490                                          | 0.4489          | 0.5596                                          | 0.5593          |
| 0.1923            | 0.4792                                          | 0.4791          | 0.6084                                          | 0.6082          |
| 0.1795            | 0.5098                                          | 0.5098          | 0.6585                                          | 0.6583          |
| 0.1667            | 0.5409                                          | 0.5409          | 0.7098                                          | 0.7096          |
| 0.1538            | 0.5725                                          | 0.5724          | 0.7625                                          | 0.7624          |
| 0.1410            | 0.6045                                          | 0.6045          | 0.8168                                          | 0.8166          |
| 0.1282            | 0.6371                                          | 0.6371          | 0.8727                                          | 0.8726          |
| 0.1154            | 0.6702                                          | 0.6702          | 0.9305                                          | 0.9304          |
| 0.1026            | 0.7039                                          | 0.7039          | 0.9903                                          | 0.9902          |
| 0.0897            | 0.7383                                          | 0.7383          | 1.0525                                          | 1.0524          |
| 0.0769            | 0.7733                                          | 0.7733          | 1.1172                                          | 1.1171          |
| 0.0641            | 0.8090                                          | 0.8090          | 1.1847                                          | 1.1847          |
| 0.0513            | 0.8455                                          | 0.8455          | 1.2557                                          | 1.2557          |
| 0.0385            | 0.8827                                          | 0.8828          | 1.3304                                          | 1.3305          |
| 0.0256            | 0.9209                                          | 0.9209          | 1.4096                                          | 1.4097          |
| 0.0128            | 0.9599                                          | 0.9600          | 1.4941                                          | 1.4942          |

## III. DATA FOR FIGURE 8

| Depolarizing prob. (p) | $\hat{E}_{\alpha(10)}^u(\mathcal{D}^P)$ (d = 2) | Analytical(d=2) | $\hat{E}_{\alpha(10)}^u(\mathcal{D}^P)$ (d = 3) | Analytical(d=3) |
|------------------------|-------------------------------------------------|-----------------|-------------------------------------------------|-----------------|
| 0.5000                 | 0.0000                                          | 0.0000          | 0.0000                                          | 0.0000          |
| 0.4872                 | 0.0000                                          | 0.0000          | 0.0000                                          | 0.0000          |
| 0.4744                 | 0.0000                                          | 0.0000          | 0.0000                                          | 0.0000          |
| 0.4615                 | 0.0000                                          | 0.0000          | 0.0000                                          | 0.0000          |
| 0.4487                 | 0.0000                                          | 0.0000          | 0.0000                                          | 0.0000          |
| 0.4359                 | 0.0000                                          | 0.0000          | 0.0000                                          | 0.0000          |
| 0.4231                 | 0.0000                                          | 0.0000          | 0.0000                                          | 0.0000          |
| 0.4103                 | 0.0000                                          | 0.0000          | 0.0000                                          | 0.0000          |
| 0.3974                 | 0.0000                                          | 0.0000          | 0.0000                                          | 0.0000          |
| 0.3846                 | 0.0000                                          | 0.0000          | 0.0000                                          | 0.0000          |
| 0.3718                 | 0.0000                                          | 0.0000          | 0.0001                                          | 0.0001          |
| 0.3590                 | 0.0000                                          | 0.0000          | 0.0013                                          | 0.0013          |
| 0.3462                 | 0.0000                                          | 0.0000          | 0.0043                                          | 0.0043          |
| 0.3333                 | 0.0000                                          | 0.0000          | 0.0090                                          | 0.0090          |
| 0.3205                 | 0.0007                                          | 0.0007          | 0.0155                                          | 0.0155          |
| 0.3077                 | 0.0029                                          | 0.0029          | 0.0238                                          | 0.0237          |
| 0.2949                 | 0.0065                                          | 0.0065          | 0.0339                                          | 0.0339          |
| 0.2821                 | 0.0116                                          | 0.0116          | 0.0459                                          | 0.0458          |
| 0.2692                 | 0.0183                                          | 0.0183          | 0.0598                                          | 0.0598          |
| 0.2564                 | 0.0266                                          | 0.0265          | 0.0758                                          | 0.0757          |
| 0.2436                 | 0.0364                                          | 0.0364          | 0.0939                                          | 0.0938          |
| 0.2308                 | 0.0480                                          | 0.0480          | 0.1141                                          | 0.1140          |
| 0.2179                 | 0.0614                                          | 0.0613          | 0.1366                                          | 0.1365          |
| 0.2051                 | 0.0765                                          | 0.0765          | 0.1616                                          | 0.1615          |
| 0.1923                 | 0.0937                                          | 0.0936          | 0.1891                                          | 0.1890          |
| 0.1795                 | 0.1129                                          | 0.1128          | 0.2194                                          | 0.2192          |
| 0.1667                 | 0.1343                                          | 0.1342          | 0.2526                                          | 0.2524          |
| 0.1538                 | 0.1580                                          | 0.1579          | 0.2890                                          | 0.2888          |
| 0.1410                 | 0.1843                                          | 0.1842          | 0.3289                                          | 0.3287          |
| 0.1282                 | 0.2135                                          | 0.2134          | 0.3727                                          | 0.3725          |
| 0.1154                 | 0.2458                                          | 0.2456          | 0.4210                                          | 0.4207          |
| 0.1026                 | 0.2816                                          | 0.2814          | 0.4742                                          | 0.4739          |
| 0.0897                 | 0.3215                                          | 0.3213          | 0.5332                                          | 0.5329          |
| 0.0769                 | 0.3661                                          | 0.3660          | 0.5992                                          | 0.5989          |
| 0.0641                 | 0.4167                                          | 0.4165          | 0.6738                                          | 0.6735          |
| 0.0513                 | 0.4746                                          | 0.4744          | 0.7594                                          | 0.7592          |
| 0.0385                 | 0.5425                                          | 0.5423          | 0.8604                                          | 0.8602          |
| 0.0256                 | 0.6254                                          | 0.6253          | 0.9848                                          | 0.9846          |
| 0.0128                 | 0.7360                                          | 0.7359          | 1.1537                                          | 1.1536          |
| 0.0000                 | 0.9999                                          | 1.0000          | 1.5848                                          | 1.5850          |
